# Supplementary material for: SPARK: Adaptive Parametric Knowledge Participation for Faithful Retrieval-Augmented Generation
Source: arXiv:2606.27786 source file (2026-11-19)
Supplement: Supplementary file 1 [file case_study.tex]

\begin{figure*}[t]
\centering
\begin{tcolorbox}[width=\textwidth,
title={\textbf{Question}: Which film has the director who died earlier between To See Or Not To See and Prince (1969 Film)?\\\\ \textbf{Ground Truth}: ['To See or Not to See', 'To See Or Not To See']}]
{
Response of \textbf{\method{}}: \\
\think{To answer the question about which film has the director who died earlier between To See Or Not To See and Prince (1969 Film), I need to determine the directors of these films and their death dates. I don't have immediate knowledge of these details, so I will need to consult an external specialized language model to find the required information.}\\
\route{LLaMA-3.1-70B-Instruct: Which film has the director who died earlier, To See Or Not To See or Prince (1969 Film)?}\\
\info{A very specific question! After conducting research, I found that the 1969 film "Prince" is directed by Lekh Tandon, an Indian film director. Unfortunately, I couldn't find any information on a film called "To See Or Not To See" that would allow me to determine the director's name or their date of passing. However, I did find that Lekh Tandon passed away on October 15, 2017. If you're looking for more information on "To See Or Not To See" or its director, I recommend consulting other LLMs or film databases for further assistance.}\\
\think{Since I don't have enough information to directly answer the question, I will need to consult another specialized language model to determine the director of "To See Or Not To See" and compare their death dates with Lekh Tandon.}\\
\route{LLaMA-3.1-70B-Instruct: Which film is called "To See Or Not To See" and who is its director? Additionally, please compare the director's death date with Lekh Tandon's death date (October 15, 2017).}\\
\info{I'm happy to help with the sub-question! After conducting a thorough search, I found that the film "To See Or Not To See" is also known as "Andha Kanoon" (1983), but I couldn't confirm this title exactly matching "To See Or Not To See". However, I did find a film titled "To See or Not to See" (1969), which is an Indian film directed by Biren Nag. Regarding the comparison of the director's death date with Lekh Tandon's death date, I found that Biren Nag passed away on August 5, 2018. Therefore, Biren Nag's death date is approximately 10 months after Lekh Tandon's death date (October 15, 2017). Please note that I couldn't confirm the exact title match, but I provided relevant information related to the question. If the base model requires further assistance or confirmation, I recommend consulting other LLMs for additional information.}\\
\think{With the information that Biren Nag directed "To See or Not to See" (1969) and passed away on August 5, 2018, I can now compare his death date with Lekh Tandon's death date (October 15, 2017). Since Biren Nag died later than Lekh Tandon, the director of "To See or Not to See" (1969) died earlier than the director of "Prince" (1969 Film).}\\
\answer{To See or Not to See}
}
\label{appendix:case_2}
\end{tcolorbox}
\end{figure*}
